# Supplementary material for: Fast and reliable confidence intervals for a variance component
Source: arXiv:2404.15060 ancillary file (2024-11-02)
Supplement: Supplementary file 1 [file supp_plain.pdf]

# Supplementary material to “Fast and reliable confidence intervals for a variance component”

Yiqiao Zhang<sup>\*</sup>   Karl Oskar Ekvall<sup>\*,†</sup>   Aaron J. Molstad<sup>‡</sup>

<sup>\*</sup>Department of Statistics, University of Florida

<sup>†</sup>Division of Biostatistics, Institute of Environmental Medicine, Karolinska Institutet

<sup>‡</sup>School of Statistics, University of Minnesota

yiqiaozhang@ufl.edu   k.ekvall@ufl.edu   amolstad@umn.edu

November 1, 2024

## A Proofs

*Proof of Proposition 1.* We first derive a convenient expression for the stochastic part of the restricted score function. Recall  $P = \Sigma^{-1/2}X(X^T\Sigma^{-1}X)^{-1}X^T\Sigma^{-1/2}$  and write  $Y - X\tilde{\beta} = Y - X(X^T\Sigma^{-1}X)^{-1}X^T\Sigma^{-1}Y = (I_n - X(X^T\Sigma^{-1}X)^{-1}X^T\Sigma^{-1})Y = (I_n - \Sigma^{1/2}P\Sigma^{-1/2})Y$ . Thus,

$$\begin{aligned} (Y - X\tilde{\beta})^T\Sigma^{-1}V_j\Sigma^{-1}(Y - X\tilde{\beta}) &= Y^T(I_n - \Sigma^{-1/2}P\Sigma^{1/2})\Sigma^{-1}V_j\Sigma^{-1}(I_n - \Sigma^{1/2}P\Sigma^{-1/2})Y \\ &= Y^T\Sigma^{-1/2}(I_n - P)\Sigma^{-1/2}V_j\Sigma^{-1/2}(I_n - P)\Sigma^{-1/2}Y \\ &= Y^T\Sigma^{-1/2}Q\Sigma^{-1/2}V_j\Sigma^{-1/2}Q\Sigma^{-1/2}Y. \end{aligned}$$

Since  $Q\Sigma^{-1/2}X = \Sigma^{-1/2}X - \Sigma^{-1/2}X(X^T\Sigma^{-1}X)^{-1}X^T\Sigma^{-1}X = \Sigma^{-1/2}X - \Sigma^{-1/2}X = 0$ , the preceding display has the same distribution as

$$\xi_n^T Q \Sigma^{-1/2} V_j \Sigma^{-1/2} Q \xi_n,$$

where  $\xi_n \sim N(0, I_n)$  and the distribution holds jointly for  $j \in \{1, 2\}$ . For  $j = 1$  we get

$$\begin{aligned} Q\Sigma^{-1/2}V_1\Sigma^{-1/2}Q &= Q\Sigma^{-1/2}O\sigma_n^2(\Lambda - I_n)O^T\Sigma^{-1/2}Q \\ &= QO\{h^2\Lambda + (1 - h^2)I_n\}^{-1/2}(\Lambda - I_n)\{h^2\Lambda + (1 - h^2)I_n\}^{-1/2}OQ \\ &= QHQ, \end{aligned}$$

and, similarly,  $Q\Sigma^{-1/2}V_2\Sigma^{-1/2}Q = Q\Sigma^{-1/2}(\Sigma/\sigma^2)\Sigma^{-1/2}Q = Q/\sigma^2$ . It follows that

$$\begin{aligned} \mathcal{I}_{11}(h^2, \sigma^2) &= \frac{1}{2} \text{tr}(QHQQHQ) = \frac{1}{2} \text{tr}(QHQQH) \\ \mathcal{I}_{12}(h^2, \sigma^2) &= \frac{1}{2} \text{tr}(QHQQ/\sigma^2) = \frac{1}{2\sigma^2} \text{tr}(QH) \\ \mathcal{I}_{22}(h^2, \sigma^2) &= \frac{1}{2\sigma^4} \text{tr}(Q) = \frac{n - p}{2\sigma^4}. \end{aligned}$$

□

*Proof of Theorem 1.* We start with some useful observations. First,  $\mathcal{I}_{11}(h^2, \sigma^2) = \text{tr}(QHQQHQ)/2$  and  $\mathcal{I}_{12}(h^2, \sigma^2) = \text{tr}(QHQQ)/(2\sigma^2)$  since  $Q$  is idempotent. Secondly, the eigenvalues of  $QHQQ$  are real since  $QHQQ$  is symmetric, and hence the eigenvalues of  $QHQQHQ$  are positive as the squares of real numbers.

Now, suppose  $QHQQ$  has  $n - p$  eigenvalues equal to some  $c \in \mathbb{R}$ , with the remaining  $p$  eigenvalues equal to zero. Then the determinant

$$|\mathcal{I}(h^2, \sigma^2)| = \frac{1}{4\sigma^4} \{(n - p) \text{tr}(QHQQHQ) - \text{tr}(QHQQ)^2\}$$

is zero since  $\text{tr}(QHQQHQ) = (n - p)c^2$  and  $\text{tr}(QHQQ) = (n - p)c$ . Thus,  $\mathcal{I}(h^2, \sigma^2)$  is singular.

To establish the other direction, suppose instead that not all of the  $n - p$  possibly non-zero eigenvalues of  $QHQQ$  are identical. Then Jensen's inequality gives

$$\frac{1}{n - p} \sum_{i=1}^n \gamma_i(QHQQ)^2 > \left\{ \frac{1}{n - p} \sum_{i=1}^n \gamma_i(QHQQ) \right\}^2,$$

where  $\gamma_i(\cdot)$  is the  $i$ th largest eigenvalue. Thus,  $|\mathcal{I}(h^2, \sigma^2)| > 0$ . Moreover, at least one eigenvalue of  $QHQQHQ$  is strictly positive, so  $\mathcal{I}_{11}(h^2, \sigma^2) > 0$ . Thus,  $\mathcal{I}(h^2, \sigma^2)$  is positive definite by Sylvester's criterion. □

**Lemma A.** *If (1) holds for some  $X$  with full column rank, then*

$$(n - p)\tilde{\sigma}^2(h^2)/\sigma_n^2 \sim \chi_{n-p}^2.$$

*Proof.* Assuming  $O = I_n$ , by (9) and proof of Proposition 1,

$$\begin{aligned} (n - p)\tilde{\sigma}^2(h^2)/\sigma_n^2 &= (Y - X\tilde{\beta})^T \Sigma^{-1} (Y - X\tilde{\beta}) \\ &= Y^T (I_n - \Sigma^{-1/2} P \Sigma^{1/2}) \Sigma^{-1} (I_n - \Sigma^{1/2} P \Sigma^{-1/2}) Y \\ &= Y^T \Sigma^{-1/2} (I_n - P) \Sigma^{1/2} \Sigma^{-1} \Sigma^{1/2} (I_n - P) \Sigma^{-1/2} Y \\ &= Y^T \Sigma^{-1/2} (I_n - P) (I_n - P) \Sigma^{-1/2} Y \\ &= Y^T \Sigma^{-1/2} Q \Sigma^{-1/2} Y. \end{aligned}$$

Since  $Q \Sigma^{-1/2} X = 0$  given by proof of Proposition 1,  $Q \Sigma^{-1/2} Y \sim \mathcal{N}(0, Q)$ , then the above quadratic form has the same distribution as  $\xi_n^T Q \xi_n$ , where  $\xi_n \sim \mathcal{N}(0, I_n)$ .

By spectral decomposition,  $Q = C \Omega C^T$  for some orthogonal  $C \in \mathbb{R}^{n \times n}$  and  $\Omega = \text{diag}(1, \dots, 1, 0, \dots, 0)$  with rank  $n - p$ . Since  $C^T \xi_n \sim \mathcal{N}(0, I_n)$ , we can write

$$\xi_n^T Q \xi_n = \xi_n^T C \Omega C^T \xi_n = (C^T \xi_n)^T \Omega (C^T \xi_n) = \sum_{i=1}^{n-p} (C^T \xi_n)_i^2 \sim \chi_{n-p}^2,$$

where  $(C^T \xi_n)_i$  is the  $i$ th element of  $C^T \xi_n$ . □

*Proof of Lemma 1.* We write  $\mathcal{I}_n = \mathcal{I}_n(h_n^2, \sigma_n^2)$  and  $U_n = U(h_n^2, \sigma_n^2)$  for simplicity. By continuous mapping theorem, it suffices to show

$$\mathcal{J}_n^{-1/2} \mathcal{D}_n^{-1} U_n \rightsquigarrow N(0, I_2), \quad (1)$$

where  $\mathcal{I}_n = \mathcal{D}_n \mathcal{J}_n \mathcal{D}_n$ ,  $\mathcal{J}_n$  is the correlation matrix corresponding to  $\mathcal{I}_n$ , and  $\mathcal{D}_n$  is diagonal with positive entries. By definition,  $\mathcal{J}_n$  is the covariance matrix of  $\mathcal{D}_n^{-1} U_n$ . Also, from Proposition 1,  $\mathcal{D}_{n11} = \|QH Q\|_F / \sqrt{2}$  and  $\mathcal{D}_{n22} = \sqrt{(n-p)} / (\sqrt{2} \sigma_n^2)$ .

To prove (1), it suffices to show that (i) the eigenvalues of  $\mathcal{J}_n$  are bounded away from zero and infinity asymptotically, and (ii) for any unit-length  $w \in \mathbb{R}^2$ ,

$$\frac{w^T \mathcal{D}_n^{-1} U_n}{\text{var}(w^T \mathcal{D}_n^{-1} U_n)^{1/2}} = \frac{w^T \mathcal{D}_n^{-1} U_n}{(w^T \mathcal{J}_n w)^{1/2}} \rightsquigarrow N(0, 1). \quad (2)$$

We start with (ii). By arguments in the proof of Proposition 1,

$$\begin{aligned} \sqrt{2} w^T \mathcal{D}_n^{-1} U_n &\sim w_1 \xi_n^T (Q_n H_n Q_n / \|Q_n H_n Q_n\|_F) \xi_n - w_1 \text{tr}(Q_n H_n Q_n / \|Q_n H_n Q_n\|_F) \\ &\quad + w_2 \xi_n^T Q_n \xi_n / \sqrt{n-p} - w_2 \text{tr}(Q_n / \sqrt{n-p}) \\ &= \xi_n^T \left( w_1 \frac{Q_n H_n Q_n}{\|Q_n H_n Q_n\|_F} + w_2 \frac{Q_n}{\sqrt{n-p}} \right) \xi_n - w_1 \text{tr} \left( \frac{Q_n H_n Q_n}{\|Q_n H_n Q_n\|_F} \right) \\ &\quad - w_2 \sqrt{n-p} \\ &= \xi_n^T K_n \xi_n - \text{tr}(K_n), \end{aligned}$$

where  $K_n$  is defined by the last equality. Using spectral decomposition of  $K_n$  and rotational invariance of the normal distribution,

$$\xi_n^T K_n \xi_n - \text{tr}(K_n) \sim \sum_{i=1}^{n-p} \gamma_i(K_n) (\xi_{ni}^2 - 1).$$

We establish (2) by verifying Lyapunov's condition (Billingsley, 1995, Theorem 27.3) holds for the right-hand side in the last display. Let

$$a_n = \sum_{i=1}^n \mathbb{E}[\{\gamma_i(K_n) (\xi_{ni}^2 - 1)\}^2] = \mathbb{E}\{(\xi_{11}^2 - 1)^2\} \sum_{i=1}^n \gamma_i(K_n)^2 = \mathbb{E}\{(\xi_{11}^2 - 1)^2\} \|K_n\|_F^2$$

and

$$b_n = \sum_{i=1}^n \mathbb{E}[\{\gamma_i(K_n) (\xi_{ni}^2 - 1)\}^4] = \mathbb{E}\{(\xi_{11}^2 - 1)^4\} \sum_{i=1}^n \gamma_i(K_n)^4 \leq \mathbb{E}\{(\xi_{11}^2 - 1)^4\} \|K_n\|^2 \|K_n\|_F^2.$$

Lyapunov's condition says (2) holds if  $b_n/a_n^2 \rightarrow 0$ , which holds if and only if  $\|K_n\|/\|K_n\|_F \rightarrow 0$ . We next show  $\|K_n\| \rightarrow 0$  and  $\liminf_{n \rightarrow \infty} \|K_n\|_F > 0$ .

For the former we have, by the triangle inequality and submultiplicativity of the spectral norm,

$$\begin{aligned}\|K_n\| &\leq |w_1| \frac{\|Q_n H_n Q_n\|}{\|Q_n H_n Q_n\|_F} + |w_2| \frac{\|Q_n\|}{\sqrt{n-p}} = |w_1| \frac{\|H_n\|}{\|Q_n H_n Q_n\|_F} + |w_2| \frac{1}{\sqrt{n-p}} \\ &= |w_1| \frac{\gamma_1(D_n^2)^{1/2}}{\|Q_n H_n Q_n\|_F} + |w_2| \frac{1}{\sqrt{n-p}},\end{aligned}$$

which tends to zero by assumption 2 since, by H.1.h of Marshall et al. (2011),

$$\begin{aligned}\|Q_n H_n Q_n\|_F^2 &= \text{tr}(Q_n H_n Q_n H_n) \\ &= \text{tr}(H_n Q_n H_n - P_n H_n Q_n H_n) \\ &= \text{tr}(H_n^2 - H_n P_n H_n - P_n H_n^2 + P_n H_n P_n H_n) \\ &\geq \text{tr}(H_n^2) - 2 \text{tr}(P_n H_n^2) \\ &\geq \text{tr}(D_n^2) - 2 \sum_{i=1}^p \gamma_i(D_n^2).\end{aligned}$$

To show  $\liminf_{n \rightarrow \infty} \|K_n\|_F > 0$  we consider two cases. First, if  $|w_1| \neq |w_2|$ , then by reverse triangle inequality,

$$\begin{aligned}\left\| w_1 \frac{Q_n H_n Q_n}{\|Q_n H_n Q_n\|_F} + w_2 \frac{Q_n}{\sqrt{n-p}} \right\|_F &\geq \left| \left\| w_1 \frac{Q_n H_n Q_n}{\|Q_n H_n Q_n\|_F} \right\|_F - \left\| w_2 \frac{Q_n}{\sqrt{n-p}} \right\|_F \right| \\ &= ||w_1| - |w_2||,\end{aligned}\tag{3}$$

which is greater than zero and does not depend on  $n$ . If instead  $|w_1| = |w_2|$ ,

$$\begin{aligned}\left\| w_1 \frac{Q_n H_n Q_n}{\|Q_n H_n Q_n\|_F} + w_2 \frac{Q_n}{\sqrt{n-p}} \right\|_F^2 &= w_1^2 \left\| \frac{Q_n}{\sqrt{n-p}} \pm \frac{Q_n H_n Q_n}{\|Q_n H_n Q_n\|_F} \right\|_F^2 \\ &= w_1^2 \text{tr} \left( \frac{Q_n^2}{n-p} + \frac{(Q_n H_n Q_n)^2}{\|Q_n H_n Q_n\|_F^2} \pm 2 \frac{Q_n}{\sqrt{n-p}} \frac{Q_n H_n Q_n}{\|Q_n H_n Q_n\|_F} \right) \\ &= 2w_1^2 \left\{ 1 \pm \text{tr} \left( \frac{Q_n}{\sqrt{n-p}} \frac{Q_n H_n Q_n}{\|Q_n H_n Q_n\|_F} \right) \right\},\end{aligned}\tag{4}$$

so, since  $Q_n$  is idempotent, it suffices to show

$$\limsup_{n \rightarrow \infty} \frac{|\text{tr}(Q_n H_n)|}{\sqrt{n-p} \|Q_n H_n Q_n\|_F} < 1.$$

We bound the numerator first. By the triangle inequality,

$$|\text{tr}(Q_n H_n)| = |\text{tr}(H_n) - \text{tr}(P_n H_n)| \leq |\text{tr}(H_n)| + |\text{tr}(P_n H_n)|.$$

Applying H.1.g and H.1.h of Marshall et al. (2011) (note their comment regarding positive semi-definiteness) to  $\text{tr}(P_n H_n)$ , we have

$$\sum_{i=1}^p \gamma_{n-p+i}(D_n) \leq \text{tr}(P_n H_n) \leq \sum_{i=1}^p \gamma_i(D_n),\tag{5}$$

which gives an upper bound of  $|\text{tr}(P_n H_n)|$ . Using this bound followed by Jensen's inequality gives

$$\begin{aligned} |\text{tr}(P_n H_n)| &\leq \max \left\{ \left| \sum_{i=1}^p \gamma_i(D_n) \right|, \left| \sum_{i=1}^p \gamma_{n-p+i}(D_n) \right| \right\} \\ &\leq \sum_{i=1}^p \sqrt{\gamma_i(D_n^2)} \\ &\leq \left( p \sum_{i=1}^p \gamma_i(D_n^2) \right)^{1/2}. \end{aligned}$$

We thus have that the ratio to be bounded is no greater than

$$\frac{|\text{tr}(D_n)| + \{p \sum_{i=1}^p \gamma_i(D_n^2)\}^{1/2}}{\sqrt{n-p} \{\text{tr}(D_n^2) - 2 \sum_{i=1}^p \gamma_i(D_n^2)\}^{1/2}} = \frac{|\text{tr}(D_n)|}{\sqrt{n-p} \{\text{tr}(D_n^2) - 2 \sum_{i=1}^p \gamma_i(D_n^2)\}^{1/2}} + o(1).$$

By assumption 2, and since  $n/(n-p) \rightarrow 1$  by assumption 1, the last right-hand side is

$$\{1 + o(1)\} \frac{n^{-1/2} |\text{tr}(D_n)|}{\text{tr}(D_n^2)^{1/2}} + o(1),$$

the upper limit of which is less than one by assumption 3, which establishes (2).

It remains only to establish (i). First, since  $\mathcal{J}_n$  is a correlation matrix, its entries are no greater than one in absolute value, and hence  $\gamma_1(\mathcal{J}_n) = \|\mathcal{J}_n\| \leq \|\mathcal{J}_n\|_F \leq 2$ . To bound  $\gamma_2(\mathcal{J}_n)$  away from zero, suppose for contradiction  $\liminf_{n \rightarrow \infty} \gamma_2(\mathcal{J}_n) = 0$ . Then we can pick a subsequence along which  $\gamma_2(\mathcal{J}_n) \rightarrow 0$ . Since  $\|\mathcal{J}_n\|_F$  is bounded, we may also, by the Bolzano–Weierstrass property, pick the subsequence in such a way that  $\mathcal{J}_n$  converges to some positive semi-definite  $\mathcal{J}$ . Since  $\gamma_2(\mathcal{J}_n) \rightarrow 0$ ,  $\mathcal{J}$  has at least one vanishing eigenvalue. Let  $w$  be a corresponding eigenvector. Then, along the subsequence,  $w^T \mathcal{J}_n w \rightarrow 0$ . But, by the arguments following (2),  $w^T \mathcal{J}_n w = \|K_n\|_F^2$ , and we already proved  $\liminf_{n \rightarrow \infty} \|K_n\|_F > 0$ , which gives the desired contradiction. Thus, (i) holds and the proof is complete.  $\square$

*Proof of Lemma 2.* Define a remainder  $R_{n1}$  to be dealt with later by

$$U_{n1}(h_n^2, \tilde{\sigma}_n^2) = U_{n1}(h_n^2, \sigma_n^2) + \nabla_{12}^2 l_R(h_n^2, \sigma_n^2)(\tilde{\sigma}_n^2 - \sigma_n^2) + R_{n1}.$$

Since

$$U_{n2}(h_n^2, \sigma_n^2) = -\frac{n-p}{2\sigma_n^2} + \frac{(n-p)\tilde{\sigma}_n^2}{2\sigma_{np}^4},$$

we have  $\tilde{\sigma}_n^2 - \sigma_n^2 = 2\sigma_{np}^4 U_{n2}(h_n^2, \sigma_n^2)/(n-p) = U_{n2}/\mathcal{I}_{n22}(h_n^2, \sigma_n^2)$ . For the remainder of the proof, we omit the arguments when they are the true parameters  $(h_n^2, \sigma_n^2)$ . Then

$$U_{n1}(h_n^2, \tilde{\sigma}_n^2) = U_{n1} + (\nabla_{12}^2 l_R) U_{n2}/\mathcal{I}_{n22} + R_{n1} = U_{n1} - \mathcal{I}_{n12} \mathcal{I}_{n22}^{-1} U_{n2} + R_{n1} + R_{n2},$$

where  $R_{n2} = (\nabla_{12}^2 l_R + \mathcal{I}_{n12})U_{n2}/\mathcal{I}_{n22}$ . We complete the proof by showing (i)  $R_{n1}^2 \mathcal{I}_n^{(11)} \rightarrow 0$  in probability, (ii)  $R_{n2}^2 \mathcal{I}_n^{(11)} \rightarrow 0$  in probability, and (iii)

$$\{U_{n1} - \mathcal{I}_{n12}U_{n2}/\mathcal{I}_{n22}\}(\mathcal{I}_n^{(11)})^{1/2} \rightsquigarrow N(0, 1).$$

It will be useful to note

$$\mathcal{I}_n^{(11)} = (\mathcal{I}_{n11} - \mathcal{I}_{n21}^2/\mathcal{I}_{n22})^{-1} = \frac{\mathcal{I}_{n22}}{\mathcal{I}_{n11}\mathcal{I}_{n22} - \mathcal{I}_{n21}^2},$$

which in fact does not depend on  $\sigma_n^2$ . We begin with (ii) and have

$$\begin{aligned} \nabla_{12}^2 l_R &= \nabla_1 U_{n2} = -\frac{1}{2\sigma_{np}^4} \sum_{i=1}^n \frac{(\lambda_i - 1)(Y_i - X_i^T \tilde{\beta})^2}{(h_n^2 \lambda_i + 1 - h_n^2)^2} \\ &= -\frac{1}{2\sigma_n^2} (Y - X\tilde{\beta})^T \Sigma_n^{-1/2} D_n \Sigma_n^{-1/2} (Y - X\tilde{\beta}) \end{aligned}$$

From the proof of Proposition 1,  $Y - X\tilde{\beta} = (I_n - \Sigma_n^{1/2} P \Sigma_n^{-1/2})Y = \Sigma_n^{1/2} (I_n - P_n) \Sigma_n^{-1/2} Y = \Sigma_n^{1/2} Q_n \Sigma_n^{-1/2} Y$ , and so

$$\nabla_{12}^2 l_R = -\frac{1}{2\sigma_n^2} Y^T \Sigma_n^{-1/2} Q_n D_n Q_n \Sigma_n^{-1/2} Y.$$

Thus,  $-R_{n2}(\mathcal{I}_n^{(11)})^{1/2}$  is

$$\frac{1}{2n^{-1/2} \sigma_n^2 (\mathcal{I}_{n11} \mathcal{I}_{n22} - \mathcal{I}_{n12}^2)^{1/2}} \frac{1}{n^{1/2}} (Y^T \Sigma_n^{-1/2} Q_n D_n Q_n \Sigma_n^{-1/2} Y - \text{tr}(Q_n D_n)) U_{n2} / \sqrt{\mathcal{I}_{n22}},$$

which we can write as  $I^{-1/2} \times II \times III$  by defining

$$\begin{aligned} I &= 4n^{-1} \sigma_{np}^4 (\mathcal{I}_{n11} \mathcal{I}_{n22} - \mathcal{I}_{n12}^2) = \text{tr}(Q_n D_n Q_n D_n) \left\{ 1 - p/n - \frac{n^{-1} \text{tr}(Q_n D_n)^2}{\text{tr}(Q_n D_n Q_n D_n)} \right\}; \\ II &= \frac{1}{n^{1/2}} (Y^T \Sigma_n^{-1/2} Q_n D_n Q_n \Sigma_n^{-1/2} Y - \text{tr}(Q_n D_n)); \\ III &= \frac{U_{n2}}{\sqrt{\mathcal{I}_{n22}}}. \end{aligned}$$

By calculations in the proof of Lemma 1, the term of I in curly brackets is bounded away from zero asymptotically (c.f. condition 3 of that lemma), so  $I \geq c \text{tr}(Q_n D_n Q_n D_n)$  for some  $c > 0$  and all large enough  $n$ . Next, II has mean zero and variance  $\text{tr}(Q_n D_n Q_n D_n)/n$ . Thus,  $I^{-1/2} \times II$  has mean zero and variance no greater than  $1/(cn)$ , and hence it tends to zero in mean square and probability. By Chebyshev's inequality, III is  $O_P(1)$ , and hence  $I^{-1/2} \times II \times III \rightarrow 0$  in probability, which completes the proof of (ii).

To show (i), use that, by Taylor's theorem with Lagrange-form remainder, for some  $\bar{\sigma}_{np}^2$  between  $\sigma_n^2$  and  $\tilde{\sigma}_{np}^2$ ,

$$R_{n1} = \nabla_{122}^3 l_R (h_n^2, \bar{\sigma}_{np}^2) (\tilde{\sigma}_{np}^2 - \sigma_n^2)^2 / 2.$$

Using calculations similar to when deriving  $\nabla_{12}^2 l_R$ , we get

$$\nabla_{122}^3 l_R(h_n^2, \bar{\sigma}_{np}^6) = \frac{1}{2\bar{\sigma}_{np}^6} \sum_{i=1}^n \frac{(\lambda_i - 1)(Y_i - X_i^T \tilde{\beta})^2}{(h_n^2 \lambda_i + 1 - h_n^2)^2} = \frac{\sigma_n^2}{2\bar{\sigma}_{np}^6} Y^T \Sigma_n^{-1/2} Q_n D_n Q_n \Sigma_n^{-1/2} Y.$$

Thus,  $2R_{n1}(\mathcal{I}_n^{(11)})^{1/2}$  is

$$\begin{aligned} & \frac{\sigma_n^6}{\bar{\sigma}_{np}^6} \frac{1}{2\sigma_{np}^4} \frac{\mathcal{I}_{n22}^{1/2}}{(\mathcal{I}_{n11}\mathcal{I}_{n22} - \mathcal{I}_{n12}^2)^{1/2}} Y^T \Sigma_n^{-1/2} Q_n D_n Q_n \Sigma_n^{-1/2} Y (U_{n2}/\mathcal{I}_{n22})^2 \\ &= \frac{\sigma_n^6}{\bar{\sigma}_{np}^6} \frac{n^{-1/2}}{2\sigma_n^2 n^{-1/2} (\mathcal{I}_{n11}\mathcal{I}_{n22} - \mathcal{I}_{n12}^2)^{1/2}} Y^T \Sigma_n^{-1/2} Q_n D_n Q_n \Sigma_n^{-1/2} Y \frac{U_{n2}^2}{\mathcal{I}_{n22}} \frac{\mathcal{I}_{n22}^{1/2}}{\mathcal{I}_{n22}\sigma_n^2} \\ &= \frac{\sigma_n^6}{\bar{\sigma}_{np}^6} \frac{n^{-1/2}}{\mathbf{I}^{1/2}} Y^T \Sigma_n^{-1/2} Q_n D_n Q_n \Sigma_n^{-1/2} Y \times \text{III}^2 \times \frac{\sqrt{2}}{\sqrt{n-p}} \\ &= \frac{\sigma_n^6}{\bar{\sigma}_{np}^6} \times \mathbf{I}^{-1/2} \times (\mathbf{II} + \text{tr}(Q_n D_n)/\sqrt{n}) \times \text{III}^2 \times \frac{\sqrt{2}}{\sqrt{n-p}}. \end{aligned}$$

Note  $|\bar{\sigma}_{np}^2/\sigma_n^2 - 1| \leq |\tilde{\sigma}_n^2/\sigma_n^2 - 1|$  and  $\tilde{\sigma}_n^2/\sigma_n^2 \sim \chi_{n-p}^2/(n-p)$ , which tends to 1 in probability. Thus,  $\bar{\sigma}_{np}^2/\sigma_n^2$  tends to one in probability and, by the arguments used to establish (ii), it suffices to show  $|\text{tr}(Q_n D_n)/n| \times \mathbf{I}^{-1/2} \rightarrow 0$ . But Jensen's inequality applied to the sum of the  $n$  real eigenvalues of  $QDQ$ , which are the same as those of  $QD$ , gives  $|\text{tr}(Q_n D_n)/n| \leq \text{tr}(Q_n D_n Q_n D_n)^{1/2} n^{-1/2}$  and in the proof of (ii) we argued  $\mathbf{I} \geq c \text{tr}(Q_n D_n Q_n D_n)$ , so

$$|\text{tr}(Q_n D_n)/n| \times \mathbf{I}^{-1/2} \leq (cn)^{-1/2} \rightarrow 0.$$

Finally, to show (iii), let  $a_n = (\mathcal{I}_n^{(11)})^{1/2}[1, -\mathcal{I}_{n12}/\mathcal{I}_{n22}]^T$ , so that what we want to show is  $a_n^T U_n \rightsquigarrow N(0, 1)$ . A direct calculation shows the variance of  $a_n^T U_n$  is  $a_n^T \mathcal{I}_n a_n = 1$ . Let  $b_n = \mathcal{I}_n^{1/2} a_n$ . Then  $\|b_n\| = 1$  and  $a_n^T U_n = b_n^T \mathcal{I}_n^{-1/2} U_n$ . The proof of Lemma 1 shows  $\mathcal{I}_n^{-1/2} U_n \rightsquigarrow N(0, I_2)$ . Moreover, by the Bolzano–Weierstrass Theorem and the subsequence principle, we may assume  $b_n \rightarrow b$  for some  $b$  with  $\|b\| = 1$ . The Cramér–Wold Theorem says  $b^T \mathcal{I}_n^{-1/2} U_n \rightsquigarrow N(0, 1)$ , and therefore  $b_n^T \mathcal{I}_n^{-1/2} U_n = b^T \mathcal{I}_n^{-1/2} U_n + (b_n - b)^T \mathcal{I}_n^{-1/2} U_n = b^T \mathcal{I}_n^{-1/2} U_n + o_P(1) \rightsquigarrow N(0, 1)$  by Slutsky's Theorem, which completes the proof.  $\square$

*Proof of Theorem 2.* Condition 1 is the same as in Lemma 1, so it suffices to verify the remaining conditions of Lemma 1. First, condition 3 ensures

$$\liminf_{n \rightarrow \infty} \min_{i \in \{1, \dots, n\}} \{h_n^2(\lambda_{ni} - 1) + 1\} > 0,$$

so together with condition 2 we have, for some  $c_{\max} \in (0, \infty)$ ,

$$\limsup_{n \rightarrow \infty} \sqrt{\gamma_1(D_n^2)} = \limsup_{n \rightarrow \infty} \max_{i \in \{1, \dots, n\}} \left| \frac{\lambda_{ni} - 1}{h_n^2(\lambda_{ni} - 1) + 1} \right| \leq c_{\max}. \quad (6)$$

Condition 2 also implies we may upon increasing  $c_{\max}$  if needed have, for any  $\lambda_{ni}$  and  $\lambda_{nj}$ ,

$$0 < (h_n^2(\lambda_{ni} - 1) + 1)(h_n^2(\lambda_{nj} - 1) + 1) \leq \max\{1, \lambda_{ni}\} \max\{1, \lambda_{nj}\} \leq c_{\max}^2.$$

Thus, if  $|\lambda_{ni} - \lambda_{nj}| > \epsilon$ ,

$$\left| \frac{\lambda_{ni} - 1}{h_n^2(\lambda_{ni} - 1) + 1} - \frac{\lambda_{nj} - 1}{h_n^2(\lambda_{nj} - 1) + 1} \right| = \frac{|\lambda_{ni} - \lambda_{nj}|}{(h_n^2(\lambda_{ni} - 1) + 1)(h_n^2(\lambda_{nj} - 1) + 1)} > \frac{\epsilon}{c_{\max}^2}. \quad (7)$$

Thus, if two diagonal elements of  $\Lambda_n$  are more than  $\epsilon$  apart, then the corresponding diagonal elements of  $D_n$  are more than  $\epsilon/c_{\max}^2$  apart.

Applying (7) with  $\lambda_{nj} = 1$  shows the number of eigenvalues of  $D_n$  in  $[-\epsilon/(c_{\max}^2), \epsilon/(c_{\max}^2)]$  is at most  $k_n^1$ , the number of eigenvalues of  $\Lambda_n$  in  $[1 - \epsilon, 1 + \epsilon]$ . Consequently, together with condition 1 we have

$$\frac{\sum_{i=1}^p \gamma_i(D_n^2)}{\sum_{i=1}^n \gamma_i(D_n^2)} \leq \frac{pc_{\max}^2}{(n - k_n^1)\epsilon^2/c_{\max}^4} \rightarrow 0,$$

which verifies condition 2 of Lemma 1.

Let  $\bar{\gamma}_n = \frac{1}{n} \sum_{i=1}^n \gamma_i(D_n)$  and let  $r_n$  be the number of eigenvalues of  $D_n$  in  $[\bar{\gamma}_n - \epsilon/(4c_{\max}^2), \bar{\gamma}_n + \epsilon/(4c_{\max}^2)]$ . Then

$$\sum_{i=1}^n \gamma_i(D_n^2) - n\bar{\gamma}_n^2 = \sum_{i=1}^n \{\gamma_i(D_n) - \bar{\gamma}_n\}^2 \geq \frac{\epsilon^2}{16c_{\max}^4}(n - r_n).$$

We are done if  $\limsup_{n \rightarrow \infty} r_n/n < 1$  since, then, condition 3 of Lemma 1 is satisfied:

$$\limsup_{n \rightarrow \infty} \frac{\text{tr}(D)^2}{n \text{tr}(D^2)} = 1 - \liminf_{n \rightarrow \infty} \frac{\sum_{i=1}^n \gamma_i(D_n^2) - n\bar{\gamma}_n^2}{\sum_{i=1}^n \gamma_i(D_n^2)} \leq 1 - \liminf_{n \rightarrow \infty} \frac{\epsilon^2 n}{16c_{\max}^6(n - r_n)} < 1.$$

To see  $r_n/n$  is indeed bounded away from one, observe  $\bar{\gamma}_n$  is bounded by (6), so we may, by the Bolzano–Weierstrass property and passing to a subsequence if necessary, assume  $\bar{\gamma}_n$  converges to some  $\gamma_0 \in \mathbb{R}$ . Thus, for all large enough  $n$ , all the eigenvalues of  $D_n$  in  $[\bar{\gamma}_n - \epsilon/(4c_{\max}^2), \bar{\gamma}_n + \epsilon/(4c_{\max}^2)]$  are also in  $[\gamma_0 - \epsilon/(2c_{\max}^2), \gamma_0 + \epsilon/(2c_{\max}^2)]$ . But then, by (7), the corresponding  $\lambda_{ni}$  are in  $[\lambda_0 - \epsilon, \lambda_0 + \epsilon]$  for some fixed  $\lambda_0$ . For example, we can fix any  $i$  and  $n$  such that  $\gamma_i(D_n) \in [\gamma_0 - \epsilon/(2c_{\max}^2), \gamma_0 + \epsilon/(2c_{\max}^2)]$  and let  $\lambda_0$  be the corresponding  $\lambda_{ni}$ . Thus,  $r_n \leq k_n^{\lambda_0}$  and the proof is completed since  $\limsup_{n \rightarrow \infty} k_n^{\lambda_0}/n < 1$  by condition 4.  $\square$

## B Different parameterizations and models

Recall  $h^2 = \sigma_g^2/(\sigma_g^2 + \sigma_e^2)$  and  $\sigma^2 = \sigma_g^2 + \sigma_e^2$ . Thus, the Jacobian of the vector  $[h^2, \sigma^2]^T$  as a function of  $(\sigma_g^2, \sigma_e^2)$  is

$$J = \begin{bmatrix} \frac{\partial h^2}{\partial \sigma_g^2} & \frac{\partial h^2}{\partial \sigma_e^2} \\ \frac{\partial \sigma^2}{\partial \sigma_g^2} & \frac{\partial \sigma^2}{\partial \sigma_e^2} \end{bmatrix} = \begin{bmatrix} \frac{\sigma_e^2}{(\sigma_g^2 + \sigma_e^2)^2} & -\frac{\sigma_g^2}{(\sigma_g^2 + \sigma_e^2)^2} \\ 1 & 1 \end{bmatrix}.$$

This Jacobian has full rank; its determinant  $1/(\sigma_g^2 + \sigma_e^2)$  is strictly positive for all possible parameter values. Thus, the score for  $[\sigma_g^2, \sigma_e^2]^\top$  is  $J^\top U$ , where  $U$  is the score for  $[h^2, \sigma^2]^\top$ , and the corresponding Fisher information is  $J^\top \mathcal{I} J$ . Because  $J$  is invertible, the test-statistic for  $[\sigma_g^2, \sigma_e^2]^\top$  is  $(J^\top U)^\top (J^\top \mathcal{I} J)^{-1} J^\top U = U^\top \mathcal{I}^{-1} U = T_n^R$ .

The parameters in Crainiceanu and Ruppert (2004) are  $\tau = \sigma_g^2/\sigma_e^2$  and  $\sigma_e^2$ . This gives  $h^2 = \tau/(1 + \tau)$  and  $\sigma^2 = \sigma_e^2(1 + \tau)$ , with the Jacobian

$$\tilde{J} = \begin{bmatrix} (1 + \tau)^{-1} & 0 \\ \sigma_e^2 & 1 + \tau \end{bmatrix}.$$

This Jacobian has determinant  $(1 + \tau)^{-1} > 0$ . Thus, the test-statistic for  $[\tau, \sigma_e^2]^\top$  is the same as that for  $[h^2, \sigma_e^2]^\top$  and that for  $[\sigma_g^2, \sigma_e^2]^\top$ . These arguments show the conclusions of Lemma 1 and Theorem 1 of the main manuscript hold in either of the three parameterizations considered. More generally, the conclusions hold after any differentiable reparameterization with full rank Jacobian. Moreover, because  $h^2$  is a strictly increasing function of  $\tau$ , a valid confidence interval for one gives, by a transformation of the endpoints, a valid confidence interval for the other.

Natural extensions of the considered model would be to assume (i)  $\Sigma = \sum_{j=1}^r \sigma_j^2 K_j$  for some known covariance matrices  $K_1, \dots, K_r$  and variance components  $\sigma_1^2, \dots, \sigma_r^2$ , or (ii) that  $\Sigma = \sigma_e I_n + \sigma_g^2 K(\zeta)$  for some parameter  $\zeta$ .

Under (i), suppose we want a confidence interval for  $h_r^2 = \sigma_r^2 / \sum_{j=1}^r \sigma_j^2$ , for example. Then  $\sigma^2 = \sum_{j=1}^r \sigma_j^2$  and  $h_j^2 = \sigma_j^2 / \sigma^2$ ,  $j \in \{1, \dots, r-1\}$  are effectively nuisance parameters. We are able to deal with the former by using that the corresponding partial maximizer of the likelihood,  $\tilde{\sigma}^2$ , is positive with probability one, and in particular is asymptotically normal under the null hypothesis; this follows from Lemma A. By contrast, partial maximizers corresponding to the nuisance  $h_j^2$  can be zero, and will be so with appreciable probability if the parameters are close to zero. Thus, those partial maximizers are not asymptotically normal under the null hypothesis, for the same reason maximum likelihood estimators of parameters near or at the boundary are not asymptotically normal in general. Results similar to Lemma 2 in the main manuscript would require new theory under sequences of nuisance parameters tending to the boundary. We are aware of no suitable results in the literature, and establishing them is a substantial undertaking and an avenue for future research.

For (ii), suppose  $\zeta$  is identifiable and of fixed dimension as  $n$  grows. Let  $U_1(h^2, \sigma^2, \zeta)$  be the restricted score for  $h^2$  and  $\mathcal{I}(h^2, \sigma^2, \zeta)$  the restricted information matrix. Let  $(\tilde{\sigma}^2, \tilde{\zeta})(h^2)$  be a partial maximizer of the restricted likelihood for a fixed  $h^2$ . A result similar to Lemma 2 of the main manuscript could be established for the test-statistic  $U_1(h^2, \tilde{\sigma}^2(h), \tilde{\zeta}(h^2))^2 \mathcal{I}^{11}(h^2, \tilde{\sigma}^2(h), \tilde{\zeta}(h^2))$  under additional conditions. However, the conditions would have to include  $\sigma_g^2 \neq 0$ , and hence  $h^2 \neq 0$ , since otherwise the distribution of  $Y$  does not depend on  $K$ , making estimation of  $\zeta$  impossible. Consequently, reliable inference under (ii) is not possible in general in the boundary settings we consider. Conversely, if the boundary problem is removed, for example by considering only sequences of parameters tending to interior points, then results like Lemma 2 should hold for all common versions of Wald, score, and likelihood ratio-statistics by classical arguments (Cox and Hinkley, 2000,

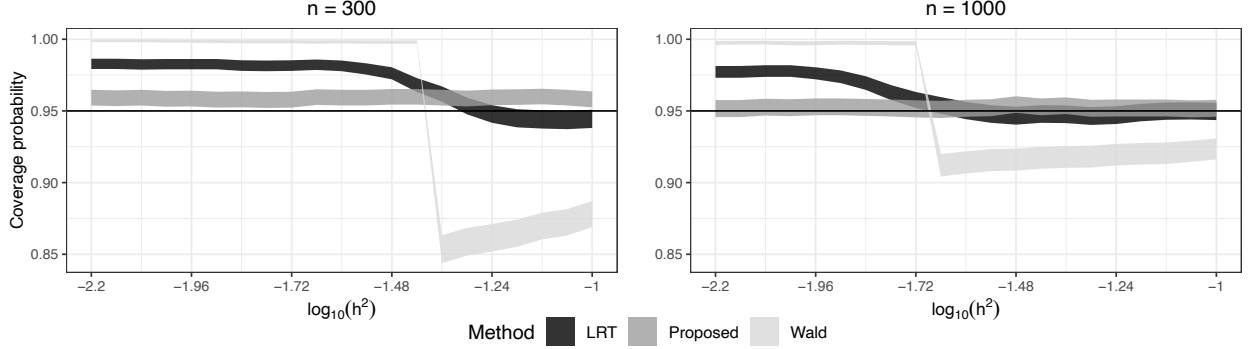

Figure 1: Monte Carlo estimates of coverage probabilities for  $h^2$  with  $\sigma_g^2 + \sigma_e^2 = 1$ ,  $\beta = 0$ ,  $X \in \mathbb{R}^{n \times 5}$  a matrix of independent standard normal entries, and  $K_{ij} = 0.95^{|i-j|}$ . The solid horizontal line indicates the nominal level, 0.95. The line widths provide 95% confidence bands for the coverage probability based on  $10^4$  trials.

Section 9.3), with some modifications to account for the fact that the parameter depends on the sample size.

## C Additional numerical results

In Fig. 1, we display simulation-based estimates of the coverage probabilities from Fig. 1 of the main manuscript, but over a smaller interval for  $h^2$ . In Fig. 1, the likelihood ratio test has coverage above the nominal level when  $\log_{10}(h^2) \leq -1.24$  with  $n = 300$ , but with  $n = 1000$ , maintains the nominal coverage level at  $\log_{10}(h^2) = -1.48$ . The Wald interval's coverage as a function of  $h^2$  also differs from  $n = 300$  to  $n = 1000$ .

In Fig. 2, we display a comparison of our proposed interval's width to the width of the interval proposed in Schweiger et al. (2016) (i.e., ALBI). Based on 1000 independent replications under the same data generating scheme used in the main manuscript's numerical studies, we see that with  $n = 200$  and  $h^2$  close to zero, the ALBI interval can be more narrow than our interval on average. However, with  $n = 500$  or larger, we saw that our intervals tend to be more narrow, on average, for almost every considered combination of  $h^2$  and  $n$ .

Though not displayed here, we found the coverage probabilities of the ALBI interval to be close to the nominal level in every considered scenario. This is expected as, like the other simulation-based methods, ALBI simulates from the exact distribution of the test-statistic, and hence the coverage probability should be correct up to Monte Carlo error.

## References

Billingsley, P. (1995). *Probability and Measure*. Wiley series in probability and mathematical statistics. Wiley, New York, 3rd ed edition.

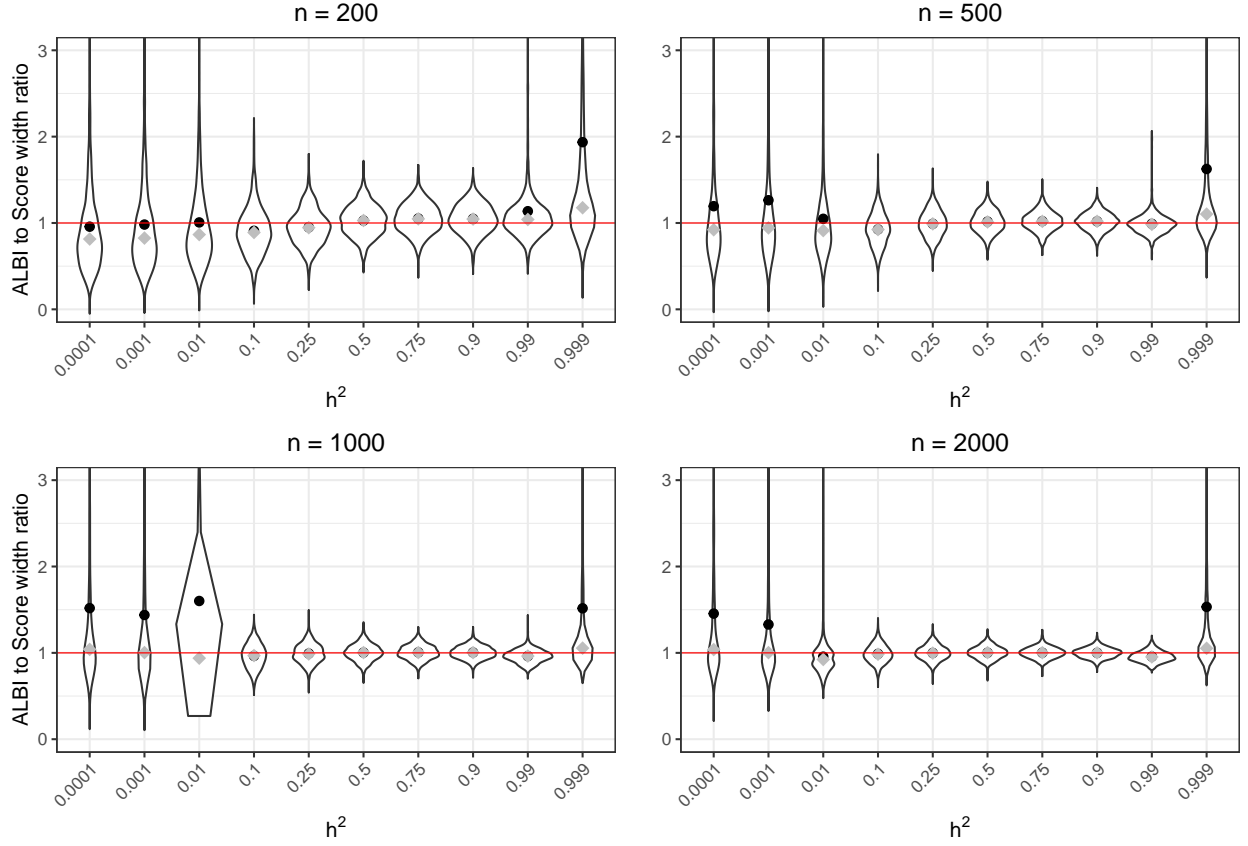

Figure 2: Violin plots of the ratio of the width of the interval proposed in Schweiger et al. (2016) to our interval's width with  $\sigma_g^2 + \sigma_e^2 = 1$ ,  $\beta = 0$ ,  $X \in \mathbb{R}^{n \times 5}$  a matrix of independent standard normal entries, and  $K_{ij} = 0.95^{|i-j|}$ . Black dots (resp. grey diamonds) indicate the mean (resp. median) ratio over 1000 independent replications.

- Cox, D. R. and Hinkley, D. V. (2000). *Theoretical Statistics*. Chapman & Hall/CRC, Boca Raton.
- Crainiceanu, C. M. and Ruppert, D. (2004). Likelihood ratio tests in linear mixed models with one variance component. *Journal of the Royal Statistical Society: Series B (Statistical Methodology)*, 66(1):165–185.
- Marshall, A. W., Olkin, I., and Arnold, B. C. (2011). *Inequalities: Theory of Majorization and Its Applications*. Springer series in statistics. Springer Science+Business Media, LLC, New York, 2nd ed edition.
- Schweiger, R., Kaufman, S., Laaksonen, R., Kleber, M. E., März, W., Eskin, E., Rosset, S., and Halperin, E. (2016). Fast and accurate construction of confidence intervals for heritability. *The American Journal of Human Genetics*, 98(6):1181–1192.
